# Supplementary material for: HiNoVa: A Novel Open-Set Detection Method for Automating RF Device Authentication
Source: arXiv:2305.09594 source file (2023-05-16)
Supplement: Supplementary file 1 [file appendix.tex]

\begin{table}[h]
\centering

\caption{Avg. test set AUPRC Values for Different Hidden Nodes and Hist. Bins - LoRa Dataset}
\label{tab:auprc}
\begin{tabular}{|c|c|c|c|c|}
\hline
\textbf{Hidden Nodes} & \textbf{Hist. Bins} & \textbf{Avg. AUPRC \algo} & \textbf{Avg. AUPRC \algoc} & \textbf{Avg. AUPRC CNN+LSTM Max Conf.} \\
\hline
\multirow{4}{*}{32} & 25 & 0.87 & 0.77 & 0.35 \\
& 50 & 0.87 & 0.72 & 0.35 \\
& 75 & 0.87 & 0.67 & 0.35 \\
& 100 & 0.87 & 0.66 & 0.35 \\
\hline
\multirow{4}{*}{64} & 25 & 0.89 & 0.83 & 0.36 \\
& 50 & 0.89 & 0.82 & 0.36 \\
& 75 & 0.89 & 0.78 & 0.36 \\
& 100 & 0.88 & 0.70 & 0.36 \\
\hline
\multirow{4}{*}{128} & 25 & 0.87 & 0.85 & 0.37 \\
& 50 & 0.87 & 0.81 & 0.37 \\
& 75 & 0.88 & 0.74 & 0.37 \\
& 100 & 0.89 & 0.71 & 0.37 \\
\hline
\end{tabular}
\end{table}

\begin{table}[h]
\centering

\caption{Avg. test set AUPRC Values for Different Hidden Nodes and Hist. Bins - Wired-WiFi Dataset}
\label{tab:auprc2}
\begin{tabular}{|c|c|c|c|c|}
\hline
\textbf{Hidden Nodes} & \textbf{Hist. Bins} & \textbf{Avg. AUPRC \algo} & \textbf{Avg. AUPRC \algoc} & \textbf{Avg. AUPRC CNN+LSTM Max Conf.} \\
\hline
\multirow{4}{*}{32} & 25 & 0.91 & 0.84 & 0.51 \\
& 50 & 0.91 & 0.80 & 0.51 \\
& 75 & 0.91 & 0.81 & 0.51 \\
& 100 & 0.91 & 0.78 & 0.51 \\
\hline
\multirow{4}{*}{64} & 25 & 0.91 & 0.91 & 0.49 \\
& 50 & 0.92 & 0.88 & 0.49 \\
& 75 & 0.92 & 0.86 & 0.49 \\
& 100 & 0.91 & 0.84 & 0.49 \\
\hline
\multirow{4}{*}{128} & 25 & 0.91 & 0.92 & 0.49 \\
& 50 & 0.92 & 0.88 & 0.49 \\
& 75 & 0.92 & 0.86 & 0.49 \\
& 100 & 0.92 & 0.82 & 0.49 \\
\hline
\end{tabular}
\end{table}

\begin{table}[h]
\centering

\caption{Avg. test set AUPRC Values for Different Hidden Nodes and Hist. Bins - Wireless-Wifi Dataset}
\label{tab:auprc3}
\begin{tabular}{|c|c|c|c|c|}
\hline
\textbf{Hidden Nodes} & \textbf{Hist. Bins} & \textbf{Avg. AUPRC \algo} & \textbf{Avg. AUPRC \algoc} & \textbf{Avg. AUPRC CNN+LSTM Max Conf.} \\
\hline
\multirow{4}{*}{32} & 25 & 0.98 & 0.88 & 0.63 \\
& 50 & 0.97 & 0.87 & 0.63 \\
& 75 & 0.96 & 0.86 & 0.63 \\
& 100 & 0.96 & 0.85 & 0.63 \\
\hline
\multirow{4}{*}{64} & 25 & 0.99 & 0.93 & 0.63 \\
& 50 & 0.98 & 0.91 & 0.63 \\
& 75 & 0.97 & 0.90 & 0.63 \\
& 100 & 0.96 & 0.88 & 0.63 \\
\hline
\multirow{4}{*}{128} & 25 & 0.99 & 0.93 & 0.63 \\
& 50 & 0.98 & 0.93 & 0.63 \\
& 75 & 0.97 & 0.90 & 0.63 \\
& 100 & 0.96 & 0.88 & 0.63 \\
\hline
\end{tabular}
\end{table}
